# Supplementary material for: Effect of curvature and normal forces on motor regulation of cilia
Source: arXiv:1905.04138 source file (2019-05-10)
Supplement: Supplementary file 1 [file appendixasym.tex]

%\begin{savequote}[75mm] 
%Some quote of Langevin
%\qauthor{Antoni van Leeuwenhoek, 1713} 
%\end{savequote}
%

\chapter{Fit results}

{In this appendix we collect the detailed results of fitting the experimental data.} We show the resulting fitting parameters for ten wild type and ten mbo2 mutant beats under four  different motor control mechanisms. 

\section{Additional fitting results}
The beats of ten wild type and ten mbo2 cilia were tracked using the procedure outlined in chapter 2. In the following tables we collect the main characteristics these beats, which were necessary for performing the fits.

As one can see, the main difference between mbo2 and wild type cilia resides in the mean curvature $C_0$: for wild-type the mean curvature is about twenty times larger than for mbo2 mutants. To fit the data we used the following parameters: a bending stiffness of $\kappa=400\,\pN\cdotp\um^2$, a spacing of $a=60\,\nm$, and a friction coefficients $\xi_{\rm n}=2\xi_{\rm t}=0.0034\,\pN\cdotp\s\cdotp\um^{-2}$.

For each motor model (sliding control, curvature control and normal force control) the space of parameters was constrained following the sign convention in table \ref{tab:regimes}. For normal force control, since the sliding friction ($\chi''$) seemed to be rather small, we further constrained the sign of $\gamma'$ to be negative. Finally, in all cases the basal compliance was forced to be passive, thus with positive signs  of real and imaginary part. A fourth model in of sliding control with an active base was considered, which resulted in better fits than sliding control with a passive base.
\begin{center}
\begin{tabular}{cccc}
\multicolumn{4}{c}{\text{wild-type data}}\\
\hline
 {axoneme} & $L\, (\um)$ & $f (\Hz)$ & $C_0(\text{mm}^{-1})$ \\
\hline
 1 & 10. & 73. & -250. \\
\hline
 2 & 10. & 67. & -290. \\
\hline
 3 & 10. & 70. & -210. \\
\hline
 4 & 11. & 65. & -250. \\
\hline
 5 & 11. & 68. & -220. \\
\hline
 6 & 11. & 74. & -230. \\
\hline
 7 & 11. & 65. & -240. \\
\hline
 8 & 12. & 62. & -210. \\
\hline
 9 & 12. & 64. & -220. \\
\hline
 10 & 12. & 44. & -200. \\
\hline
\end{tabular}

\begin{tabular}{cccc}
\multicolumn{4}{c}{\text{mbo2 mutant data}}\\
\hline
 {axoneme} & $L (\um)$ & $f (\Hz)$ & $C_0(\text{mm}^{-1})$ \\
\hline
 1 & 8.4 & 41. & -9.3 \\
\hline
 2 & 8.8 & 23. & -26.\\
\hline
 3 & 9. & 33. & -41. \\
\hline
 4 & 9.2 & 23. & -5.5 \\
\hline
 5 & 9.4 & 21. & -50.\\
\hline
 6 & 9.4 & 21. & -8.2 \\
\hline
 7 & 9.4 & 38 & -32. \\
\hline
 8 & 9.7 & 18. & -27. \\
\hline
 9 & 10. & 22. & -20.\\
\hline
 10 & 11. & 43. & -39.\\
\hline
\end{tabular}
\end{center}

The fitting produce was the following. For each set of parameters the critical mode was obtained, and the mean squared distance of the predicted theoretical shape $\psi^{\rm the}$ to the experimental one $\psi^{\rm exp}$ was obtained $R^2 (\psi^{\rm the},\psi^{\rm exp})$. With the Mathematica 9 FindMaximum algorithm the maxima of this function was obtained. The fit parameters used were four (plus an arbitrary amplitude which can not be determined from the linear theory) for curvature and normal force control, and two for sliding control and sliding control with an active base. Reducing the number of parameters however did not worsen the quality of the fits of curvature control. For instance, fixing $\chi''=0$ and $\beta'=0$ allowed for an average fitting score of $\sim94\%$, while it reduced the number of parameters to two.

\begin{figure}
\centering
\includegraphics {./asym_sm_allreim_wt_nccc}
\caption{\textbf{Normal force control and curvature control fits for wild-type.} Panels A1 to A10 correspond to normal force control fits, and panels B1 to B10 correspond to curvature control. The cilium labeled 3 is not shown, as it appears already in Fig.~\ref{fig:wtfits}. The parameters obtained from the twenty fits are reported in the next page in the same order as in this figure.}
\label{fig:allncccwt}
\end{figure}

\centering
\rotatebox{90}{
\begin{array}{ccccccc}
\multicolumn{7}{c}{\text{Fit results for wild-type data with normal force control}}\\
\hline
 \text{axoneme} & R^2\text{(\%)} & \chi \,(\pN /\um^2) & \gamma  & \chi _0\,(\pN /\um) & \Delta
   _{0,0}\text{ (nm)} & \Delta _{0,1}\text{ (nm)} \\
\hline
 1 & 95. & 17.\times 10^3-12.\times 10^{-6} i & 110.\times 10^{-3}+1.9 i & 88.\times 10^3+3.1\times 10^3 i & -19. & 10.-17. i \\
\hline
 2 & 94. & 16.\times 10^3-2.3\times 10^{-6} i & 120.\times 10^{-3}+1.6 i & 140.\times 10^3+3.2\times 10^3 i & -14.  & 7.2 -13.  i \\
\hline
 3 & 96. & 13.\times 10^3+2.9\times 10^3 i & 29.\times 10^{-3}+2.1 i & 140.\times 10^3+3.6\times 10^3 i & -9.8  & 4.7 -12.  i \\
\hline
 4 & 94. & 14.\times 10^3+2.2 i & 170.\times 10^{-3}+1.8 i & 3.4\times 10^3+3.3\times 10^6 i & -480. & -.57-0.37 i \\
\hline
 5 & 95. & 14.\times 10^3+3.\times 10^3 i & 25.\times 10^{-3}+2. i & 340.\times 10^3+3.6\times 10^3 i & -4.4  & 2.8\ -4.7  i \\
\hline
 6 & 94. & 22.\times 10^3+1.4\times 10^3 i & 6.4\times 10^{-9}+2.3 i & 14.\times 10^3+31.\times 10^3 i & -110.  & 4.5 -18.  i \\
\hline
 7 & 95. & 18.\times 10^3+1.1\times 10^3 i & 35.\times 10^{-3}+2. i & 71.\times 10^3+2.8\times 10^3 i & -22.  & 11. -16.  i \\
\hline
 8 & 96. & 12.\times 10^3+1.9 i & 170.\times 10^{-3}+1.9 i & 4.1\times 10^3+9.1\times 10^6 i & -350. & -0.23-0.13 i \\
\hline
 9 & 94. & 11.\times 10^3+560. i & 140.\times 10^{-3}+1.8 i & 3.1\times 10^3+3.1\times 10^6 i & -460.& -0.66-0.39 i \\
\hline
 10 & 93. & 11.\times 10^3+1.7 i & 180.\times 10^{-3}+2. i & 1.3\times 10^9+6.5\times 10^6 i & -0.001 &0.00094-0.0012 i \\
\hline
% \text{mean} & 95. & 15.\times 10^3+900. i & 97.\times 10^{-3}+1.9 i & 130.\times 10^6+2.2\times 10^6 i & -150.\times 10^{-3} &
%   3.9\times 10^{-3}-8.1\times 10^{-3} i \\
%\hline
% \text{stand dev} & 950.\times 10^{-3} & 3.4\times 10^3+1.2\times 10^3 i & 69.\times 10^{-3}+170.\times 10^{-3} i &
%   420.\times 10^6+3.3\times 10^6 i & 200.\times 10^{-3} & 4.5\times 10^{-3}+7.8\times 10^{-3} i \\
%\hline
\\
\multicolumn{7}{c}{\text{Fit results of wild-type data with curvature control}}\\
\hline
 \text{axoneme} & R^2\text{($\%$)} & \text{$\chi $ (pN /}\text{$\mu $m}^2) & \text{$\beta $ (pN)} & \chi _0\text{ (pN/$\mu $m)} &
   \Delta _{0,0}\text{ (nm)} & \Delta _{0,1}\text{ (nm)} \\
\hline
 1 & 95. & 20.\times 10^3+1.1\times 10^3 i & 4.4\times 10^{-6}-6.7\times 10^3 i & 68.\times 10^3+2.8\times
   10^3 i & -25. & 10.-17.i \\
\hline
 2 & 94. & 21.\times 10^3+1.1\times 10^3 i & 4.4\times 10^{-6}-6.8\times 10^3 i & 71.\times 10^3+2.8\times
   10^3 i & -27. & 9.2-15.i \\
\hline
 3 & 96. & 15.\times 10^3+1.8\times 10^3 i & 4.3\times 10^{-6}-6.1\times 10^3 i & 88.\times 10^3+3.5\times
   10^3 i & -16.& 6.6-16. i \\
\hline
 4 & 93. & 13.\times 10^3+3.5\times 10^3 i & 91.-5.7\times 10^3 i & 26.\times 10^3+5.2\times 10^6 i &
   -0.62 & -0.30-0.11 i \\
\hline
 5 & 95. & 13.\times 10^3+3.4\times 10^3 i & 72.-5.7\times 10^3 i & 3.1\times 10^6+5.1\times 10^3 i &
   -0.48 & 0.29-0.50 i \\
\hline
 6 & 94. & 22.\times 10^3+950. i & 130.-7.\times 10^3 i & 15.\times 10^3+25.\times 10^3 i & -110. &
   5.4-17. i \\
\hline
 7 & 95. & 11.\times 10^3+2.7\times 10^3 i & 2.-5.4\times 10^3 i & 1.4\times 10^6+33.\times 10^3 i &
   -1.1 & 0.69-1.2 i \\
\hline
 8 & 95. & 11.\times 10^3+2.\times 10^3 i & 11.-5.3\times 10^3 i & 320.\times 10^6+3.9\times 10^6 i &
   -0.0045 & 0.002-0.0053i \\
\hline
 9 & 94. & 11.\times 10^3+2.\times 10^3 i & 28.-5.2\times 10^3 i & 340.\times 10^3+9.4\times 10^6 i &
   -4.3 & -0.18-0.085 i \\
\hline
 10 & 94. & 14.\times 10^3+2.\times 10^3 i & 39.-5.7\times 10^3 i & 21.\times 10^6+210.\times 10^3 i &
   -0.063 & 0.052-0.045 i \\
\hline
% \text{mean} & 94. & 15.\times 10^3+2.1\times 10^3 i & 37.-6.\times 10^3 i & 34.\times 10^6+1.9\times 10^6 i
%   & -24. & 3.2-6.8 i \\
%\hline
% \text{stand dev} & 840.\times 10^{-3} & 4.4\times 10^3+910. i & 46.+680. i & 100.\times 10^6+3.3\times 10^6 i & 35.&
%   4.2+8.4i \\
%\hline
\end{array}
}

\begin{figure}
\centering
\includegraphics {./asym_sm_allreim_mbo2_nccc}
\caption{\textbf{Normal force control and curvature control fits for mbo2 mutant.} Panels A1 to A10 correspond to normal force control fits, and panels B1 to B10 correspond to curvature control. The cilium labeled 7 is not shown, as it appears already in Fig.~\ref{fig:mbo2fits}. The parameters obtained from the twenty fits are reported in the next page in the same order as in this figure.}
\label{fig:allncwt}
\end{figure}
\clearpage

\centering
\rotatebox{90}{
\begin{array}{ccccccc}
\multicolumn{7}{c}{\text{Fit results for mbo2 mutant data with normal force control}}\\
\hline
 \text{axoneme} & R^2\text{($\%$)} & \text{$\chi $ (pN /}\text{$\mu $m}^2)& \gamma  & \chi _0\text{ (pN/$\mu $m)} & \Delta
   _{0,0}\text{ (nm)} & \Delta _{0,1}\text{ (nm)} \\
\hline
 1 & 95. & 7.7\times 10^3-4.\times 10^{-6} i & 3.4+48. i & 3.2\times 10^3+12.\times 10^3 i & -20.&
   -53.-87. i \\
\hline
 2 & 95. & 17.\times 10^3+1.9\times 10^3 i & 25.\times 10^{-12}+21. i & 3.1\times 10^3+16.\times 10^3 i & -55.& -5.-54. i \\
\hline
 3 & 96. & 4.5\times 10^3-9.1\times 10^{-6} i & 910.\times 10^{-3}+9.5 i & 2.8\times 10^3+9.3\times 10^3 i & -99. & -110.-120. i \\
\hline
 4 & 96. & 9.9\times 10^3+2.5\times 10^3 i & 2.4\times 10^{-9}+81. i & 2.8\times 10^3+17.\times 10^3 i & -13. & -39.-54. i \\
\hline
 5 & 96. & 12.\times 10^3+2.5\times 10^3 i & 4.4\times 10^{-9}+9.2 i & 3.\times 10^3+22.\times 10^3 i & -110. & -24.-47.i \\
\hline
 6 & 96. & 11.\times 10^3+1.5\times 10^3 i & 1.1\times 10^{-9}+55. i & 2.5\times 10^3+9.8\times 10^3 i & -22.& -19.-78.i \\
\hline
 7 & 97. & 5.1\times 10^3-6.4\times 10^{-6} i & 1.4+12. i & 3.4\times 10^3+18.\times 10^3 i & -62.&
   -76.-71. i \\
\hline
 8 & 96. & 13.\times 10^3+1.6\times 10^3 i & 1.9\times 10^{-9}+17. i & 2.6\times 10^3+13.\times 10^3 i & -68. & -13.-66. i \\
\hline
 9 & 94. & 21.\times 10^3+1.8\times 10^3 i & 1.6\times 10^{-9}+26. i & 2.6\times 10^3+33.\times 10^3 i & -52. & 5.6-33. i \\
\hline
 10 & 95. & 15.\times 10^3+2.1\times 10^3 i & 1.2\times 10^{-9}+12. i & 2.6\times 10^3+38.\times 10^3 i & -100.& -9.6-28. i \\
\hline
% \text{mean} & 96. & 12.\times 10^3+1.4\times 10^3 i & 580.\times 10^{-3}+29. i & 2.9\times 10^3+19.\times 10^3 i &
%   -60.\times 10^{-3} & -34.\times 10^{-3}-64.\times 10^{-3} i \\
%\hline
% \text{stand dev} & 850.\times 10^{-3} & 5.1\times 10^3+1.\times 10^3 i & 1.1+24. i & 300.+9.6\times 10^3 i & 35.\times
%   10^{-3} & 36.\times 10^{-3}+28.\times 10^{-3} i \\
%\hline
\\
\multicolumn{7}{c}{\text{Fit results of mbo2 mutant data with curvature control}}\\
\hline
 \text{axoneme} & R^2\text{($\%$)} & \text{$\chi $ (pN /}\text{$\mu $m}^2)& \text{$\beta $ (pN)} & \chi _0\text{ (pN/$\mu $m)} &
   \Delta _{0,0}\text{ (nm)} & \Delta _{0,1}\text{ (nm)} \\
\hline
 1 & 95. & 23.\times 10^3+810. i & 59.-7.8\times 10^3 i & 3.2\times 10^3+4.2\times 10^3 i & -19. &
   5.1-47. i \\
\hline
 2 & 95. & 20.\times 10^3+1.1\times 10^3 i & 4.1-7.3\times 10^3 i & 3.1\times 10^3+11.\times 10^3 i &
   -56.& 4.3-55. i \\
\hline
 3 & 96. & 15.\times 10^3+710. i & 3.8-6.5\times 10^3 i & 13.\times 10^3+3.3\times 10^3 i & -22. &
   -0.150-63.i \\
\hline
 4 & 96. & 17.\times 10^3+6.3\times 10^3 i & 650.-6.8\times 10^3 i & 8.3\times 10^3+11.\times 10^3 i &
   -4.4 & -8.5-40. i \\
\hline
 5 & 96. & 13.\times 10^3+4.\times 10^3 i & 240.-6.2\times 10^3 i & 3.3\times 10^3+24.\times 10^3 i &
   -100. & -22.-39. i \\
\hline
 6 & 95. & 23.\times 10^3+660. i & 64.-7.5\times 10^3 i & 2.6\times 10^3+2.8\times 10^3 i & -21. &
   23. -47.  i \\
\hline
 7 & 97. & 13.\times 10^3+1.2\times 10^3 i & 1.5\times 10^{-6}-6.1\times 10^3 i & 24.\times 10^3+4.5\times
   10^3 i & -8.9  & 1.7 -46.  i \\
\hline
 8 & 96. & 16.\times 10^3+820. i & 26.-6.6\times 10^3 i & 2.6\times 10^3+6.9\times 10^3 i & -68.&
   5.7-65. i \\
\hline
 9 & 94. & 25.\times 10^3+1.7\times 10^3 i & 100.-7.5\times 10^3 i & 2.6\times 10^3+18.\times 10^3 i &
   -53. & 15.-32.i \\
\hline
 10 & 95. & 14.\times 10^3+12.\times 10^3 i & 1.3\times 10^3-6.\times 10^3 i & 3.7\times 10^3+200.\times
   10^3 i & -71. & -3.2-3.7i \\
\hline
% \text{mean} & 95. & 18.\times 10^3+2.9\times 10^3 i & 240.-6.8\times 10^3 i & 6.6\times 10^3+29.\times 10^3
%   i & -42. & 2.-44. i \\
%\hline
% \text{stand dev} & 800.\times 10^{-3} & 4.6\times 10^3+3.6\times 10^3 i & 410.+660. i & 6.9\times 10^3+61.\times 10^3 i
%   & 32.& 12.+17. i \\
%\hline
\end{array}
}

\begin{figure}
\centering
\includegraphics {./asym_sm_allreim_wt_scscab}
\caption{\textbf{Sliding control and sliding control with an active base fits for wild-type.} Panels A1 to A9 correspond to normal force control fits, and panels B1 to B9 correspond to curvature control. The cilium labeled 7 is not shown, as it appears already in Fig.~\ref{fig:mbo2fits}. The parameters obtained from the twenty fits are reported in the next page in the same order as in this figure.}
\label{fig:allncwt}
\end{figure}
\clearpage

\centering
\rotatebox{90}{
\begin{array}{cccccc}
\multicolumn{6}{c}{\text{Fit results for wild-type data with sliding control}}\\
\hline
 \text{axoneme} & R^2\text{($\%$)} & \text{$\chi $ (pN /}\text{$\mu $m}^2) & \chi _0\text{ (pN/$\mu $m)} & \Delta _{0,0}\text{ (nm)} & \Delta _{0,1}\text{ (nm)} \\
\hline
 1 & 51. & -11.\times 10^3-1.5\times 10^3 i & 2.4\times 10^3+1.6\times 10^3 i & -710.  & 20. -34. i \\
\hline
 2 & 46. & -11.\times 10^3-1.4\times 10^3 i & 2.3\times 10^3+1.5\times 10^3 i & -850. & 17. -32. i \\
\hline
 3 & 55. & -12.\times 10^3-1.3\times 10^3 i & 11.\times 10^3+1.6\times 10^3 i & -130.  & 16. -35.  i \\
\hline
 4 & 44. & -21.\times 10^3-980. i & 530.\times 10^6+870.\times 10^6 i & -0.0031 & -0.0016 +0.11\times
   10^{-3} i \\
\hline
 5 & 50. & -16.\times 10^3-1.2\times 10^3 i & 63.\times 10^3+1.7\times 10^3 i & -24.  & -0.070-20.  i \\
\hline
 6 & 53. & -16.\times 10^3-1.4\times 10^3 i & 66.\times 10^3+1.7\times 10^3 i & -23. & 2.9 -19. i \\
\hline
 7 & 48. & -11.\times 10^3-1.5\times 10^3 i & 13.\times 10^3+1.5\times 10^3 i & -120. & 13. -34.  i \\
\hline
 8 & 0. & -14.\times 10^3-610. i & 66.\times 10^3-18.\times 10^3 i & -22.  & -3.4 -18.  i \\
\hline
 9 & 49. & -16.\times 10^3-1.3\times 10^3 i & 300.\times 10^3+2.1\times 10^3 i & -4.8  & -2.9 -5.1  i \\
\hline
 10 & 39. & -16.\times 10^3-850. i & 2.6\times 10^9+4.1\times 10^9 i & -0.52\times 10^{-3} & -0.28\times 10^{-3}-6.4\times
   10^{-9} i \\
\hline
% \text{mean} & 43. & -14.\times 10^3-1.2\times 10^3 i & 310.\times 10^6+500.\times 10^6 i & -190.\times 10^{-3} &
%   6.2\times 10^{-3}-20.\times 10^{-3} i \\
%\hline
% \text{stand dev} & 16. & 3.3\times 10^3+300. i & 820.\times 10^6+1.3\times 10^9 i & 320.\times 10^{-3} & 9.\times
%   10^{-3}+14.\times 10^{-3} i \\
%\hline
\\
\multicolumn{6}{c}{\text{Fit results of wild-type data with active base}}\\
\hline
 \text{axoneme} & R^2\text{($\%$)} & \text{$\chi $ (pN /}\text{$\mu $m}^2) & \chi _0\text{ (pN/$\mu $m)} & \Delta _{0,0}\text{ (nm)} & \Delta _{0,1}\text{ (nm)} \\
\hline
 1 & 90. & -21.\times 10^3+15.\times 10^3 i & -19.\times 10^3-56.\times 10^3 i & 89.  & 63. -11.  i \\
\hline
 2 & 89. & -22.\times 10^3+16.\times 10^3 i & -21.\times 10^3-56.\times 10^3 i & 92. & 61. -9.3 i \\
\hline
 3 & 91. & -20.\times 10^3+13.\times 10^3 i & -16.\times 10^3-55.\times 10^3 i & 86. & 59. -14.  i \\
\hline
 4 & 87. & -24.\times 10^3+13.\times 10^3 i & -22.\times 10^3-55.\times 10^3 i & 74. & 50. -12. i \\
\hline
 5 & 90. & -20.\times 10^3+12.\times 10^3 i & -18.\times 10^3-55.\times 10^3 i & 82.  & 54. -13. i \\
\hline
 6 & 86. & -19.\times 10^3+9.5\times 10^3 i & -15.\times 10^3-57.\times 10^3 i & 99.  & 46. -5.7  i \\
\hline
 7 & 89. & -18.\times 10^3+11.\times 10^3 i & -18.\times 10^3-52.\times 10^3 i & 90.  & 62. -11. i \\
\hline
 8 & 88. & -20.\times 10^3+11.\times 10^3 i & -20.\times 10^3-48.\times 10^3 i & 70. & 58. -16. i \\
\hline
 9 & 87. & -17.\times 10^3+8.5\times 10^3 i & -18.\times 10^3-50.\times 10^3 i & 80. & 56.-24.  i \\
\hline
 10 & 84. & -20.\times 10^3+10.\times 10^3 i & -19.\times 10^3-47.\times 10^3 i & 69. & 54. -5.3  i \\
\hline
% \text{mean} & 88. & -20.\times 10^3+12.\times 10^3 i & -19.\times 10^3-53.\times 10^3 i & 83.\times 10^{-3} & 56.\times
%   10^{-3}-12.\times 10^{-3} i \\
%\hline
% \text{stand dev} & 2.1 & 2.1\times 10^3+2.2\times 10^3 i & 2.\times 10^3+3.5\times 10^3 i & 9.8\times 10^{-3} &
%   5.3\times 10^{-3}+5.3\times 10^{-3} i \\
%\hline
\end{array}
}

\begin{figure}
\centering
\includegraphics {./asym_sm_allreim_mbo2_scscab}
\caption{\textbf{Sliding control and sliding control with an active base fits for mbo2} Panels A1 to A10 correspond to normal force control fits, and panels B1 to B10 correspond to curvature control. The cilium labeled 7 is not shown, as it appears already in Fig.~\ref{fig:mbo2fits}. The parameters obtained from the twenty fits are reported in the next page in the same order as in this figure.}
\label{fig:allncwt}
\end{figure}
\clearpage

\centering
\rotatebox{90}{
\begin{array}{cccccc}
\multicolumn{6}{c}{\text{Fit results for mbo2 data with sliding control}}\\
\hline
 \text{axoneme} & R^2\text{($\%$)} & \text{$\chi $ (pN /}\text{$\mu $m}^2 & \chi _0\text{ (pN/$\mu $m)} & \Delta _{0,0}\text{ (nm)} & \Delta _{0,1}\text{ (nm)} \\
\hline
 1 & 74. & -20.\times 10^3-730. i & 19.\times 10^3+2.1\times 10^3 i & -3.3& 30.-34. i \\
\hline
 2 & 68. & -19.\times 10^3-510. i & 28.\times 10^3+2.\times 10^3 i & -6.2& 34.-39. i \\
\hline
 3 & 77. & -17.\times 10^3-660. i & 17.\times 10^3+2.\times 10^3 i & -16. & 35.-42. i \\
\hline
 4 & 77. & -20.\times 10^3-440. i & 44.\times 10^3+2.1\times 10^3 i & -0.83 & 24.-38. i \\
\hline
 5 & 70. & -18.\times 10^3-470. i & 29.\times 10^3+1.9\times 10^3 i & -12. & 28.-40. i \\
\hline
 6 & 77. & -18.\times 10^3-440. i & 34.\times 10^3+2.\times 10^3 i & -1.6& 37.-39. i \\
\hline
 7 & 70. & -14.\times 10^3-740. i & 8.6\times 10^3+1.8\times 10^3 i & -25. & 31.-38. i \\
\hline
 8 & 72. & -17.\times 10^3-410. i & 33.\times 10^3+1.9\times 10^3 i & -5.4& 34.-43. i \\
\hline
 9 & 64. & -18.\times 10^3-370. i & 62.\times 10^3+1.9\times 10^3 i & -2.2 & 16.-33. i \\
\hline
 10 & 68. & -17.\times 10^3-630. i & 65.\times 10^3+1.9\times 10^3 i & -4.& 7.3-28.
  i \\
\hline
% \text{mean} & 72. & -18.\times 10^3-540. i & 34.\times 10^3+2.\times 10^3 i & -7.6\times 10^{-3} & 28.\times 10^{-3}-38.\times
%   10^{-3} i \\
%\hline
% \text{stand dev} & 4.5 & 1.7\times 10^3+140. i & 19.\times 10^3+94. i & 7.7\times 10^{-3} & 9.4\times 10^{-3}+4.4\times 10^{-3} i \\
%\hline
\\
\multicolumn{6}{c}{\text{Fit results of mbo2 data with active base}}\\
\hline
 \text{axoneme} & R^2\text{($\%$)} & \text{$\chi $ (pN /}\text{$\mu $m}^2 & \chi _0\text{ (pN/$\mu $m)} & \Delta _{0,0}\text{ (nm)} & \Delta _{0,1}\text{ (nm)} \\
\hline
 1 & 93. & -24.\times 10^3+14.\times 10^3 i & -3.5\times 10^3-58.\times 10^3 i & 18.\ & 59.-13. i \\
\hline
 2 & 90. & -24.\times 10^3+13.\times 10^3 i & -4.7\times 10^3-63.\times 10^3 i & 36. & 72.-5.i \\
\hline
 3 & 95. & -20.\times 10^3+12.\times 10^3 i & -2.3\times 10^3-52.\times 10^3 i & 120.& 68.-20. i \\
\hline
 4 & 96. & -22.\times 10^3+10.\times 10^3 i & 2.4\times 10^3-60.\times 10^3 i & -15.  & 64. -15. i \\
\hline
 5 & 92. & -21.\times 10^3+12.\times 10^3 i & -4.2\times 10^3-59.\times 10^3 i & 80.  & 69. -12.  i \\
\hline
 6 & 93. & -20.\times 10^3+9.2\times 10^3 i & 4.6\times 10^3-56.\times 10^3 i & -12.  & 70. -7.9 i \\
\hline
 7 & 94. & -19.\times 10^3+13.\times 10^3 i & -9.\times 10^3-53.\times 10^3 i & 24. & 65. -16.  i \\
\hline
 8 & 92. & -20.\times 10^3+9.9\times 10^3 i & -1.\times 10^3-57.\times 10^3 i & 0.17 & 77. -7.8  i \\
\hline
 9 & 86. & -20.\times 10^3+9.1\times 10^3 i & -5.3\times 10^3-63.\times 10^3 i & 25.  & 67. -2.5  i \\
\hline
 10 & 90. & -19.\times 10^3+8.\times 10^3 i & -4.3\times 10^3-61.\times 10^3 i & 62. & 53. -13.  i \\
\hline
% \text{mean} & 92. & -21.\times 10^3+11.\times 10^3 i & -2.7\times 10^3-58.\times 10^3 i & 51.\times 10^{-3} & 66.\times
%   10^{-3}-11.\times 10^{-3} i \\
%\hline
% \text{stand dev} & 2.8 & 1.8\times 10^3+2.\times 10^3 i & 3.9\times 10^3+3.7\times 10^3 i & 59.\times 10^{-3} &
%   6.8\times 10^{-3}+5.4\times 10^{-3} i \\
%\hline
\end{array}
}
\clearpage
