# Supplementary material for: Effect of curvature and normal forces on motor regulation of cilia
Source: arXiv:1905.04138 source file (2019-05-10)
Supplement: Supplementary file 5 [file introduction_sm_doublets.pdf]

**A** $\alpha\beta$  dimer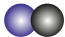

protofilament

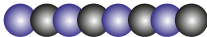

microtubule

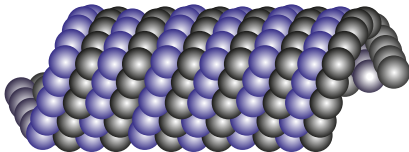**B**

axonemal doublet

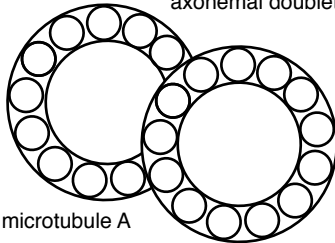

microtubule A

microtubule B
