# Supplementary material for: Effect of curvature and normal forces on motor regulation of cilia
Source: arXiv:1905.04138 source file (2019-05-10)

*Nodal cilia*

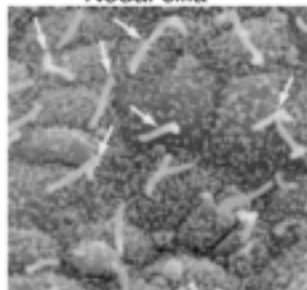

*Bronchial cilia*

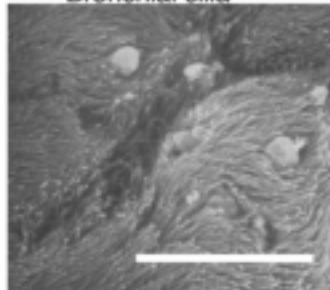

*Paramecium*

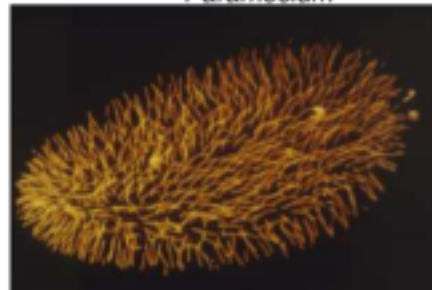

*Chlamydomonas Reinhardtii*

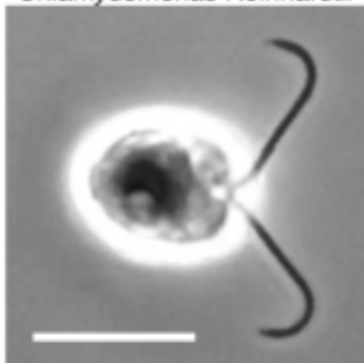

*Bull Sperm*

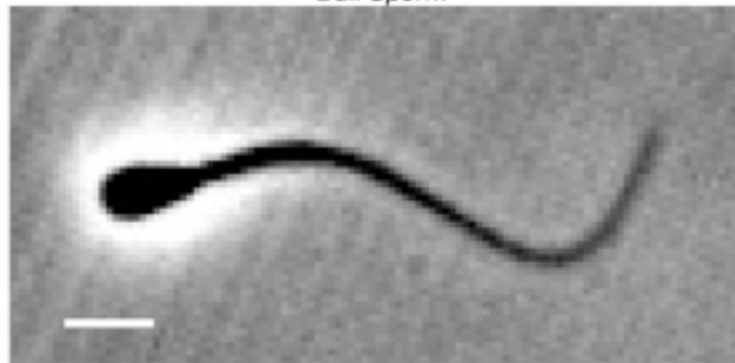

*Sea Urchin Sperm*

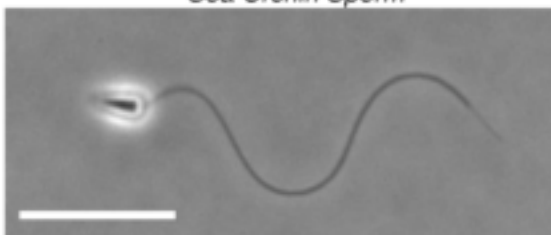

*Trypanosoma*

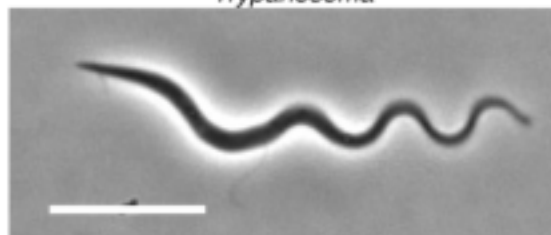

*Anopheles Sperm*

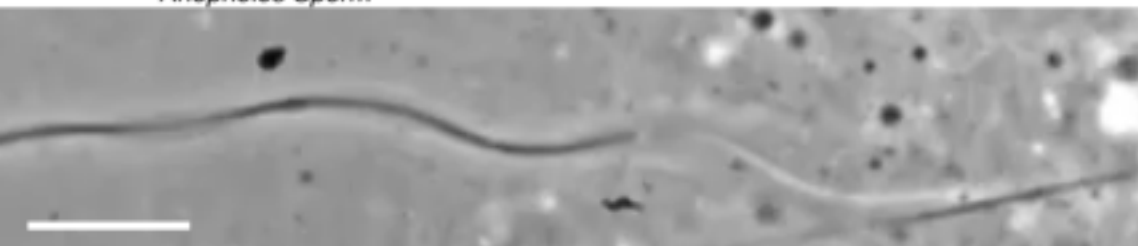

Supplement: Supplementary file 7 [file introduction_sm_flagellates_hres.pdf]
