# Supplementary material for: Effect of curvature and normal forces on motor regulation of cilia
Source: arXiv:1905.04138 source file (2019-05-10)

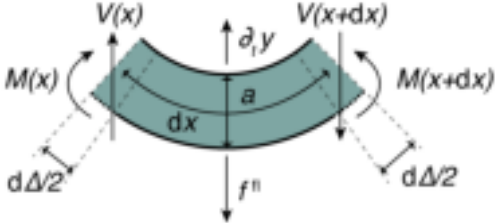

Supplement: Supplementary file 8 [file introduction_sm_freebody.pdf]
